# Supplementary material for: Randomized Nystr\"om approximation of non-negative self-adjoint operators
Source: arXiv:2404.00960 source file (2024-12-08)
Supplement: Supplementary file 2 [file finitedim_rsvd_appendix.tex]

\section{Lemmas for the finite dimensional randomized SVD}
\subsection{Imported lemmas}
Subsection containing lemmas from other papers.
\begin{lemma}[{\cite[Theorem 5.1]{multstat}}]\label{lemma:partition}
Consider
\begin{equation*}
    \begin{bmatrix} \bm{\Omega}_1 \\ \bm{\Omega}_2 \end{bmatrix} \sim N\left(\bm{0},\begin{bmatrix} \widetilde{\bm{K}}_{11}  & \widetilde{\bm{K}}_{21}^T \\ \widetilde{\bm{K}}_{21} & \widetilde{\bm{K}}_{22} \end{bmatrix}\right).
\end{equation*}
Then,
\begin{equation*}
    \bm{\Omega}_1 \sim N(\bm{0},\widetilde{\bm{K}}_{11}).
\end{equation*}
\end{lemma}

\begin{lemma}{{\cite[Theorem 5.3]{multstat}}}\label{lemma:cond_distribution}
\begin{equation*}
    \bm{\Omega}_2 | \bm{\Omega}_1 \sim N(\widetilde{\bm{K}}_{21}\widetilde{\bm{K}}_{11}^{-1} \bm{\Omega}_1, \widetilde{\bm{K}}_{22}-\widetilde{\bm{K}}_{21}\widetilde{\bm{K}}_{11}^{-1}\widetilde{\bm{K}}_{21}^T)
\end{equation*}
\end{lemma}

%\begin{lemma}{{\cite[Proposition 10.1]{rsvd}}}\label{lemma:expectation}
%Let $\bm{B}$ and $\bm{C}$ be fixed matrices and $\bm{\Psi}$ be a standard Gaussian matrix. Then
%\begin{equation*}
    %\mathbb{E}\|\bm{B\Psi C}\|_F^2 = %\|\bm{B}\|_F^2 \|\bm{C}\|_F^2.
%\end{equation*}
%\end{lemma}

\begin{lemma}{{\cite[Theorem 2.4.14]{kollo}}}\label{lemma:inversewishart_expectation}
Let $\bm{X} \sim \mathcal{W}_{m}(\bm{C},n)$. Then,
\begin{equation*}
    \mathbb{E}[\bm{X}^{-1}] = \frac{\bm{C}^{-1}}{n-m-1}.
\end{equation*}

\end{lemma}
