# Supplementary material for: Randomized Nystr\"om approximation of non-negative self-adjoint operators
Source: arXiv:2404.00960 source file (2024-12-08)
Supplement: Supplementary file 4 [file finitedim_nystrom_appendix.tex]

%\section{Lemmas for the finite dimensional symmetric Nyström approximation}\label{section:appendix}
\section{Proof of Lemma~\ref{lemma:shifted_4norm}}\label{section:lemma_shifted_4norm}
%\begin{lemma}[{\cite[Theorem 2.1]{lee}}]\label{lemma:partition_spsd}
%Let $f[0,\infty) \mapsto [0,\infty)$ be a concave function. Then, given an arbitrary partitioned positive semi-definite matrix, 
%\begin{equation*}
 %   \left\|f\left(\begin{bmatrix} \bm{A} & \bm{X}^T \\ \bm{X} & \bm{B} \end{bmatrix}\right)\right\| \leq \|f(\bm{A})\| + \|f(\bm{B})\|,
%\end{equation*}
%for any symmetric norm $\|\cdot\|$.
%\end{lemma}
\begin{lemma}\label{lemma:matrix_cube}
%Consider an $m \times n$ matrix $\bm{\Phi}$ with entries
%\begin{equation*}
%    \bm{\Phi}_{ij} = \sigma_i s_j \omega_{ij},
%\end{equation*}
%where $\sigma_i, s_j \geq 0$ and $\omega_{ij}$ are i.i.d. $N(0,1)$ random variables. Then
%\begin{equation*}
%    \mathbb{E}[\bm{\Phi}\bm{\Phi}^T \bm{\Phi}] = \bm{0}.
%\end{equation*}
Consider $\bm{C} \in \mathbb{R}^{m \times M}, \bm{D} \in \mathbb{R}^{N \times n}$ and a standard Gaussian $M \times N$ matrix $\bm{\Psi}$. Define $\bm{\Phi} = \bm{C}\bm{\bm{\Psi}}\bm{D}$. Then,
\begin{equation*}
    \mathbb{E}[\bm{\Phi}\bm{\Phi}^T \bm{\Phi}] = \bm{0}.
\end{equation*}
\end{lemma}
\begin{proof}
Let $\bm{C} = \bm{U} \bm{\Sigma} \bm{V}^T$ and $\bm{D} = \bm{Q}\bm{S}\bm{W}^T$ be the full SVDs of $\bm{C}$ and $\bm{D}$ respectively. Then, since $\bm{V}^T \bm{\Psi} \bm{Q} \stackrel{d}{=} \bm{\Psi}$ we have
\begin{equation*}
    \bm{\Phi}\bm{\Phi}^T \bm{\Phi} = \bm{U} \bm{\Sigma}\bm{\Psi} \bm{S}\bm{S}^T \bm{\Psi}^T \bm{\Sigma}^T \bm{\Sigma} \bm{\Psi} \bm{S}\bm{W}^T.
\end{equation*}
It suffices to show that
\begin{equation*}
    \mathbb{E}[\bm{\Sigma}\bm{\Psi} \bm{S}\bm{S}^T \bm{\Psi}^T \bm{\Sigma}^T \bm{\Sigma} \bm{\Psi} \bm{S}] = \bm{0}. 
\end{equation*}
Hence, let us redefine $\bm{\Phi} = \bm{\Sigma}\bm{\Psi} \bm{S}$. Note that $\bm{\Phi}_{ij} = \sigma_i s_j \psi_{ij}$ where $s_i = 0$ if $i > M$ and $s_j = 0$ if $j > N$. Note that the $(i,j)$-entry of $\bm{\Phi}\bm{\Phi}^T \bm{\Phi}$ equals
\begin{equation*}
    \bm{\Phi}(i,:) \bm{\Phi}^T \bm{\Phi}(:,j) = \sum\limits_{k=1}^n \sum\limits_{\ell = 1}^m \bm{\Phi}_{ik}\bm{\Phi}_{\ell k} \bm{\Phi}_{\ell j} = \sum\limits_{k=1}^n \sum\limits_{\ell = 1}^m \sigma_i s_j \sigma_{\ell}^2 s_k^2 \psi_{ik} \psi_{\ell k} \psi_{\ell j}.
\end{equation*}
Now note that for all $i,k,\ell$ and $j$ we have $\mathbb{E}[\psi_{ik} \psi_{\ell k} \psi_{\ell j}] = 0$, which yields the result.
\end{proof}

\begin{lemma}\label{lemma:trace_squared}
Let $\bm{B} \in \mathbb{R}^{m \times n}$ and $\bm{\Phi}$ as in Lemma~\ref{lemma:matrix_cube}. Then,
\begin{equation*}
    \mathbb{E}\tr((\bm{B}^T \bm{\Phi})^2) = \|\bm{C}^T \bm{B}\bm{D}^T \|_F^2.
\end{equation*}
\end{lemma}
\begin{proof}
Let $\bm{C}=\bm{U} \bm{\Sigma}\bm{V}^T$ and $\bm{D} = \bm{Q}\bm{S}\bm{W}^T$ be the full SVDs of $\bm{C}$ and $\bm{D}$. Hence,
\begin{equation*}
    \bm{B}^T \bm{\Phi} = \bm{U} \bm{\Sigma}\bm{V}^T\bm{\Psi} \bm{Q}\bm{S}\bm{W}^T \stackrel{d}{=}\bm{U} \bm{\Sigma}\bm{V}^T\bm{\Psi} \bm{Q}\bm{S}\bm{W}^T.
\end{equation*}
Let us redefine $\bm{\Phi} = \bm{\Sigma}\bm{\Psi}\bm{S}$. Then, if $\widetilde{\bm{B}} = \bm{U}^T \bm{B}\bm{W}$ we have
\begin{equation*}
    \mathbb{E}\tr((\bm{B}^T \bm{\Phi})^2) = \mathbb{E}\tr((\widetilde{\bm{B}}^T \bm{\Phi})^2).
\end{equation*}
Furthermore, we have
\begin{equation*}
    \mathbb{E}((\widetilde{\bm{B}}^T \bm{\Psi})^2)_{ii} = \sum\limits_{\ell = 1}^m \widetilde{\bm{B}}_{\ell i}^2 \sigma_\ell^2 s_i^2.
\end{equation*}
Hence, summing over $i$ we have
\begin{equation*}
    \mathbb{E}\tr((\bm{B}^T \bm{\Phi})^2)= \|\bm{\Sigma}^T \widetilde{\bm{B}} \bm{S}^T\|_F^2 = \|\bm{C}^T \bm{B}\bm{D}^T \|_F^2.
\end{equation*}
\end{proof}

\begin{lemma}\label{lemma:schatten4_product}
Let $\bm{\Omega}$ be a random standard Gaussian matrix. Then,
\begin{equation*}
    \mathbb{E}\|\bm{S}\bm{\Omega}\bm{Z}\|_{(4)}^4 = \|\bm{S}\|_{(4)}^4\|\bm{Z}\|_{(4)}^4 + \|\bm{S}\|_{F}^4\|\bm{Z}\|_{(4)}^4 + \|\bm{S}\|_{(4)}^4\|\bm{Z}\|_{F}^4
\end{equation*}
\end{lemma}
\begin{proof}
By unitary invariance of Schatten norms and standard Gaussian matrices we may assume without loss of generality that $\bm{S}$ and $\bm{Z}$ are diagonal matrices with non-negative diagonal entries. Let
\begin{equation*}
    \bm{B} = \bm{S}\bm{\Omega}\bm{Z}.
\end{equation*}
Then,
\begin{equation*}
    \bm{B}_{ij} = s_i z_j \omega_{ij}.
\end{equation*}
Furthermore,
\begin{equation*}
    \|\bm{B}\|_{(4)}^4 = \|\bm{B}^T \bm{B}\|_F^2.
\end{equation*}
Note that
\begin{equation*}
    (\bm{B}^T \bm{B})_{ij} = z_i z_j\sum\limits_{k}s_k^2 \omega_{ki} \omega_{kj}.
\end{equation*}
Let use denote
\begin{equation*}
    r(\bm{S}) = 2 \sum\limits_{k > \ell} s_k^2 s_{\ell}^2 = \|\bm{S}\|_F^4 - \|\bm{S}\|_{(4)}^4,
\end{equation*}
and we define $r(\bm{Z})$ similarly. We have
\begin{align*}
    &\mathbb{E}(\bm{B}^T \bm{B})_{ii}^2 = z_i^4 \left(\sum\limits_k s_k^4 \mathbb{E}\omega_{ij}^4 + 2 \sum\limits_{k > \ell} s_k^2 s_{\ell}^2 \mathbb{E}\omega_{ki}^2 \mathbb{E} \omega_{\ell j}^2\right)\\
    = & z_i^4 \left(\sum\limits_k 3 s_k^4 + 2 \sum\limits_{k > \ell} s_k^2 s_{\ell}^2 \right) = 3 z_i^4 \|\bm{S}\|_{(4)}^4 + z_i^4 r(\bm{S}).
\end{align*}
Furthermore, for $i \neq j$ we have
\begin{align*}
    &\mathbb{E}(\bm{B}^T \bm{B})_{ij}^2 = z_i^2z_j^2\left(\sum\limits_k s_k^4 \mathbb{E} [\omega_{ki}^2\omega_{kj}^2] + 2 \sum\limits_{k > \ell} s_k^2 s_{\ell}^2 \mathbb{E}[\omega_{ki}\omega_{kj}\omega_{\ell i} \omega_{\ell j}]\right)\\
    = & z_i^2 z_j^2 \|\bm{S}\|_{(4)}^4.
\end{align*}
Summing over we get
\begin{align*}
    & \mathbb{E}\|\bm{B}^T \bm{B}\|_F^2 = 3 \|\bm{Z}\|_{(4)}^4 \|\bm{S}\|_{(4)}^4 + \|\bm{Z}\|_{(4)}^4 r(\bm{S}) + \|\bm{S}\|_{(4)}^4 r(\bm{Z})\\
    = &\|\bm{S}\|_{(4)}^4\|\bm{Z}\|_{(4)}^4 + \|\bm{S}\|_{F}^4\|\bm{Z}\|_{(4)}^4 + \|\bm{S}\|_{(4)}^4\|\bm{Z}\|_{F}^4
\end{align*}
\end{proof}

\begin{lemma}[Lemma~\ref{lemma:shifted_4norm} restated.]
Consider $\bm{\Phi}$ as in Lemma~\ref{lemma:matrix_cube}. Given any matrix $\bm{B}$ we have
\begin{align*}
    &\mathbb{E}\|\bm{B}+\bm{\Phi}\|_{(4)}^4 = \|\bm{B}\|_{(4)}^4 + \mathbb{E}\|\bm{\Phi}\|_{(4)}^4 + 2( \mathbb{E}\|\bm{B}^T\bm{\Phi}\|_F^2 + \mathbb{E}\|\bm{\Phi}\bm{B}^T\|_F^2 + \mathbb{E}\tr\left((\bm{B}^T \bm{\Phi})^2\right))\\
    = & \|\bm{B}\|_{(4)}^4 + \|\bm{C}\|_{(4)}^4\|\bm{D}\|_{(4)}^4 + \|\bm{C}\|_{F}^4\|\bm{D}\|_{(4)}^4 + \|\bm{C}\|_{(4)}^4\|\bm{D}\|_{F}^4 +\\ &2\left(\|\bm{B}^T \bm{C}\|_F^2 \|\bm{D}\|_F^2 + \|\bm{C}\|_F^2 \|\bm{D}\bm{B}^T\|_F^2 + \|\bm{C}^T \bm{B}\bm{D}^T\|_F^2\right).
\end{align*}
\end{lemma}
\begin{proof}
Note that we have for any fixed matrices $\bm{C}$ and $\bm{D}$ we have $\mathbb{E}\tr(\bm{C}\bm{\Phi} \bm{D}) = 0$. This fact, together with the linearity of the trace and expectation with Lemma~\ref{lemma:matrix_cube} we have
\begin{align*}
    &\mathbb{E}\|\bm{B} + \bm{\Phi}\|_{(4)}^4 = \mathbb{E}\|(\bm{B}^T + \bm{\Phi}^T)(\bm{B} + \bm{\Phi})\|_F^2\\
    = & \mathbb{E}\|\bm{B}^T \bm{B} + \bm{B}^T \bm{\Phi} + \bm{\Phi}^T \bm{B} + \bm{\Phi}^T \bm{\Phi}\|_F^2 \\
    = & \mathbb{E}\tr((\bm{B}^T \bm{B} + \bm{B}^T \bm{\Phi} + \bm{\Phi}^T \bm{B} + \bm{\Phi}^T \bm{\Phi})(\bm{B}^T \bm{B} + \bm{B}^T \bm{\Phi} + \bm{\Phi}^T \bm{B} + \bm{\Phi}^T \bm{\Phi}))\\
    = & \|\bm{B}\|_{(4)}^4 + \mathbb{E}\|\bm{\Phi}\|_{(4)}^4 + 2( \mathbb{E}\|\bm{B}^T\bm{\Phi}\|_F^2 + \mathbb{E}\|\bm{\Phi}\bm{B}^T\|_F^2 + \mathbb{E}\tr\left((\bm{B}^T \bm{\Phi})^2\right)).
\end{align*}
The final result is obtained by applying Lemma~\ref{lemma:trace_squared} to obtain $\mathbb{E}\tr((\bm{B}^T \bm{\Psi})^2)$, Lemma~\ref{lemma:schatten4_product} to obtain $\mathbb{E}\|\bm{\Phi}\|_{4}^4$ and \cite[Proposition 10.1]{rsvd} to bound the remaining terms.
\end{proof}

%\begin{lemma}\label{lemma:shiften_4norm}
%Let $\bm{B}, \bm{C}$ and $\bm{D}$ be fixed matrices and $\bm{\Psi}$ a standard Gaussian matrix. Then,
%\begin{align*}
    %\mathbb{E}\|\bm{B} + \bm{C}\bm{\Psi}\bm{D}\|_{(4)}^4 \leq \|\bm{B}\|_{(4)} + \mathbb{E}\|\bm{C}\bm{\Psi}\bm{D}\|_{(4)}^4 + 2( \mathbb{E}\|\bm{B}^T \bm{C} \bm{\Psi}\bm{D}\|_F^2 + \mathbb{E}\|\bm{B}^T \bm{C} \bm{\Psi}\bm{D} \bm{B}^T\|_F^2 + \mathbb{E}\tr((\bm{B}^T \bm{C} \bm{\Psi}\bm{D})^2)).
%\end{align*}
%\end{lemma}
%\begin{proof}
%Let $\bm{C} = \bm{U}\bm{\Sigma} \bm{V}^T$ and $\bm{D} = \bm{Q}\bm{S}\bm{W}^T$ be the SVDs of $\bm{C}$ and $\bm{D}$ respectively. Then, by unitary invariance of Schatten norms we have
%\begin{equation*}
 %   \|\bm{B} + \bm{C}\bm{\Psi}\bm{D}\|_{(4)}^4 = \|\bm{U}^T \bm{B}\bm{W} + \bm{\Sigma}(\bm{V}^T \bm{\Psi} \bm{Q}) \bm{S}\|_{(4)}^4.
%\end{equation*}
%Note that $\bm{V}^T \bm{\Psi} \bm{Q}$ is a standard Gaussian matrix, and $\bm{\Phi} = \bm{\Sigma}(\bm{V}^T \bm{\Psi} \bm{Q}) \bm{S}$ is as in Lemma~\ref{lemma:matrix_cube}. Hence, by Lemma~\ref{lemma:shifted_4norm} we have
%\begin{align*}
 %   &\mathbb{E}\|\bm{B} + \bm{C}\bm{\Psi}\bm{D}\|_{(4)}^4 \leq \|\bm{U}^T \bm{B}\bm{W}\|_{(4)}^4 + \mathbb{E}\|\bm{\Sigma}(\bm{V}^T \bm{\Psi} \bm{Q}) \bm{S}\|_{(4)}^4 + 6 \mathbb{E}\|\bm{W}^T \bm{B}^T \bm{U} \bm{\Sigma} \bm{V}^T \bm{\Psi} \bm{Q}\bm{S}\|_F^2\\
  %  = & \|\bm{B}\|_{(4)}^4 + \mathbb{E}\|\bm{C}\bm{\Psi}\bm{D}\|_{(4)}^4 + 6 \mathbb{E}\|\bm{B}^T \bm{C}\bm{\Psi}\bm{D}\|_F^2.
%\end{align*}
%The lower bound follows from an identical argument.
%\end{proof}

\section{Proof of Lemma~\ref{lemma:inversewishart_norm_expectation}}\label{section:proof_inversewishart_norm_expectation}
\begin{lemma}[{\cite[Theorem 3.1 and Corollary 3.1]{rosen}}]\label{lemma:expectation_kronecker}
If $\bm{X} \sim \mathcal{W}_{m}(\bm{C},n)$. Then,
\begin{equation*}
    \mathbb{E}\left[\bm{X}^{-2}\right] = \frac{\bm{C}^{-2}}{(n-m)(n-m-3)} + \frac{\tr(\bm{C}^{-1}) \bm{C}^{-1}}{(n-m)(n-m-1)(n-m-3)},
\end{equation*}
and
\begin{align*}
    \mathbb{E}\left[\bm{X}^{-1} \otimes \bm{X}^{-1}\right] = \frac{(n-m-2)\bm{C}^{-1} \otimes \bm{C}^{-1}}{(n-m)(n-m-1)(n-m-3)} + \frac{\vect(\bm{C}^{-1})\vect(\bm{C}^{-1})^T}{(n-m)(n-m-1)(n-m-3)} \\+ \frac{\bm{C}_{m \times m}(\bm{C}^{-1} \otimes \bm{C}^{-1})}{(n-m)(n-m-1)(n-m-3)}
\end{align*}
where $\bm{C}_{m \times m}$ is a $m^2 \times m^2$ commutation matrix.
\end{lemma}
\begin{lemma}\label{lemma:trace_commutationmatrix}
Let $\bm{C}_{k \times k}$ be a $k^2 \times k^2$ commutation matrix, i.e. it is a $k \times k$ block matrix with $k \times k$ blocks $(\bm{C}_{k \times k})_{ij} = \bm{E}_{ji}$, where $\bm{E}_{ji}$ is a $k \times k$ with entries $(\bm{E}_{ji})_{k \ell} = \delta_{kj}\delta_{i\ell}$. Let $\bm{B}$ be a $k \times k$ symmetric matrix. Then,
\begin{equation*}
    \tr(\bm{C}_{k \times k} (\bm{B} \otimes \bm{B})) = \|\bm{B}\|_F^2.
\end{equation*}
\end{lemma}
\begin{proof}
Note that the $(i,i)-$block of $\bm{C}_{k \times k}(\bm{B} \otimes \bm{B})$ equals
\begin{align*}
    (\bm{C}_{k \times k}(\bm{B} \otimes \bm{B}))_{ii} = \sum\limits_{s = 1}^k \bm{E}_{si}\bm{B} \bm{B}_{si}.
\end{align*}
Now note that the $(j,j)-$entry of $\bm{E}_{si}\bm{B}$ equals $\delta_{sj}\bm{B}_{ij}$. Hence, $\tr(\bm{E}_{si}\bm{B}) = \bm{B}_{is} = \bm{B}_{si}$, by symmetry of $\bm{B}$. Hence,
\begin{equation*}
    \tr((\bm{C}_{k \times k}(\bm{B} \otimes \bm{B}))_{ii}) = \sum\limits_{s=1}^k \bm{B}_{si}^2.
\end{equation*}
Consequently,
\begin{equation*}
    \tr(\bm{C}_{k \times k} (\bm{B} \otimes \bm{B})) = \sum\limits_{i=1}^k \sum\limits_{s=1}^k \bm{B}_{si}^2 = \|\bm{B}\|_F^2,
\end{equation*}
as required.
\end{proof}

\begin{lemma}[Lemma~\ref{lemma:inversewishart_norm_expectation} restated]
We have
\begin{equation*}
    \mathbb{E}\|\bm{\Omega}_1^{\dagger}\|_F^4 = \frac{(p-2)\tr(\widetilde{\bm{K}}_{11}^{-1})^2 + 2 \|\widetilde{\bm{K}}_{11}^{-1}\|_F^2}{p(p-1)(p-3)},
\end{equation*}
and
\begin{equation*}
    \mathbb{E}\|\bm{\Omega}_1^{\dagger}\|_{(4)}^4 = \frac{\|\widetilde{\bm{K}}_{11}^{-1}\|_F^2}{p(p-3)} + \frac{\tr(\widetilde{\bm{K}}_{11}^{-1})^2}{p(p-1)(p-3)}.
\end{equation*}
\end{lemma}
\begin{proof}
Let $\bm{X} = \bm{\Omega}_1\bm{\Omega}_1^T \sim \mathcal{W}_k(\widetilde{\bm{K}}_{11},k+p)$. Note that by using Lemma~\ref{lemma:expectation_kronecker} we have
\begin{align*}
    &\mathbb{E}\|\bm{\Omega}_1^{\dagger}\|_F^4 = \mathbb{E}[\tr(\bm{X}^{-1})^2] = \mathbb{E}[\tr\left(\bm{X}^{-1} \otimes \bm{X}^{-1}\right)] = \tr\left(\mathbb{E}[\bm{X}^{-1} \otimes \bm{X}^{-1}]\right)\\
    = & \frac{(p-2)\tr(\widetilde{\bm{K}}_{11}^{-1} \otimes \widetilde{\bm{K}}_{11}^{-1}) + \tr(\vect(\widetilde{\bm{K}}_{11}^{-1})\vect(\widetilde{\bm{K}}_{11}^{-1})^T) + \tr(\bm{C}_{k \times k} (\widetilde{\bm{K}}_{11}^{-1} \otimes \widetilde{\bm{K}}_{11}^{-1})) }{p(p-1)(p-3)}\\
    = & \frac{(p-2)\tr(\widetilde{\bm{K}}_{11}^{-1})^2 + 2 \|\widetilde{\bm{K}}_{11}^{-1}\|_F^2}{p(p-1)(p-3)},
\end{align*}
where we used Lemma~\ref{lemma:trace_commutationmatrix} in the final step. To obtain the second equality we use Lemma~\ref{lemma:expectation_kronecker} to obtain
\begin{equation*}
    \mathbb{E}\|\bm{\Omega}_1^{\dagger}\|_{(4)}^4 = \mathbb{E}\|\bm{X}^{-1}\|_F^2 = \mathbb{E}\tr(\bm{X}^{-2}) = \frac{\|\widetilde{\bm{K}}_{11}^{-1}\|_F^2}{p(p-3)} + \frac{\tr(\widetilde{\bm{K}}_{11}^{-1})^2}{p(p-1)(p-3)}
\end{equation*}
\end{proof}

\section{Proof of Lemma~\ref{lemma:omega1_tailbound}}\label{appendix:proof_omega1_tailbounds}
\begin{lemma}[Part of Lemma~\ref{lemma:omega1_tailbound} restated]
Let $p \geq 4$. Then for $t > 1$,
\begin{align*}
    & \mathbb{P}\left(\|\bm{\Omega}_1^{\dagger}\|_{(4)} > \frac{e \sqrt{(k+p) \|\widetilde{\bm{K}}_{11}^{-1}\|_F}}{p+1} t\right) \leq t^{-(p+1)};\\
    & \mathbb{P}\left(\|\bm{\Omega}_1^{\dagger}\|_{2} > \frac{e \sqrt{(k+p) \|\widetilde{\bm{K}}_{11}^{-1}\|_2}}{p+1} t\right) \leq t^{-(p+1)}.
\end{align*}
\end{lemma}
\begin{proof}
Note that 
\begin{equation*}
    \bm{\Omega}_1^{\dagger}  \stackrel{d}{=} \bm{\Psi}^T \widetilde{\bm{K}}_{11}^{1/2}(\widetilde{\bm{K}}_{11}^{1/2}\bm{\Psi}\bm{\Psi}^T\widetilde{\bm{K}}_{11}^{1/2})^{-1} = \bm{\Psi}^T(\bm{\Psi}\bm{\Psi}^T)^{-1} \widetilde{\bm{K}}_{11}^{-1/2} = \bm{\Psi}^{\dagger}\widetilde{\bm{K}}_{11}^{-1/2}.
\end{equation*}
So for $s \in [2,\infty]$
\begin{align*}
    &\mathbb{P}\left(\|\bm{\Omega}_1^{\dagger}\|_{(s)} > \frac{e \sqrt{(k+p) \|\widetilde{\bm{K}}_{11}^{-1}\|_{(s/2)}}}{p+1} t\right) = \mathbb{P}\left(\|\bm{\Psi}_1^{\dagger} \widetilde{\bm{K}}_{11}^{-1/2}\|_{(s)} > \frac{e \sqrt{(k+p) \|\widetilde{\bm{K}}_{11}^{-1}\|_{(s/2)}}}{p+1} t\right)\\
    \leq & \mathbb{P}\left(\|\bm{\Psi}_1^{\dagger}\|_2 \|\widetilde{\bm{K}}_{11}^{-1}\|_{(s/2)}^{1/2} > \frac{e \sqrt{(k+p) \|\widetilde{\bm{K}}_{11}^{-1}\|_{(s/2)}}}{p+1} t\right) = \mathbb{P}\left(\|\bm{\Psi}_1^{\dagger}\|_2 > \frac{e \sqrt{(k+p)}}{p+1} t\right).
\end{align*}
The final result is obtained by applying \cite[Proposition 10.4]{rsvd}.
\end{proof}
